# Supplementary material for: Suns-V$_\textrm{OC}$ characteristics of high performance kesterite solar cells
Source: arXiv:1406.2326 ancillary file (2014-06-09)
Supplement: Supplementary file 1 [file SunsVoc_SupplMater08a.pdf]

# Suns-$V_{OC}$ characteristics of high performance kesterite solar cells

Oki Gunawan, Tayfun Gokmen, David B. Mitzi

*IBM T. J. Watson Research Center, PO Box 218, Yorktown Heights, NY 10598 USA*

# SUPPLEMENTAL MATERIALS

## *A. Suns-$V_{OC}$ and Suns-$I_{SC}$ measurement*

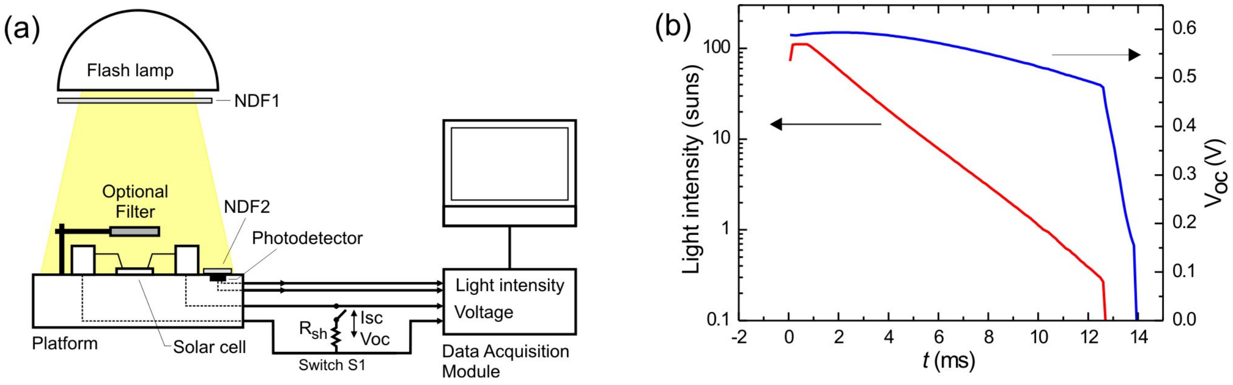


**Figure S1.** (a) Modified Sinton tool setup for Suns-$V_{OC}$ and Suns-$I_{SC}$ measurement. (b) Transient traces of the high light intensity (measured by the photodetector covered by NDF2) and the $V_{OC}$.

The modified Sinton tool setup is shown in Figure S1(a). Besides the standard function of measuring the Suns-$V_{OC}$ curve at low light intensity (up to ~1 sun), it can also measure within a higher light intensity range (up to ~ 300 suns) and measure the short circuit current ($I_{SC}$). The flash lamp is lowered to achieve higher light intensity at the solar cell-under-test. NDF1 is a set of neutral density filters (made on printed plastic films) that comes as a standard component with the Sinton tool. NDF2 is a stack of neutral density filters with total attenuation factor about 100x (or optical density 2). NDF2 is used to attenuate the light coming to the photodetector at high light intensity to avoid saturation of the photodetector signal read out.

We use two intensity setups: (1) A standard/low light intensity setup (~0.001 to 1 suns) where the neutral density filter #1 (NDF1) is inserted and no NDF2. (2) High light intensity setup (~0.3 to 300 suns) where NDF1 is removed and NDF2 covers the photodetector. An example of the standard and high light intensity Suns-$V_{OC}$ measurement is shown in Figure S3. In each of these setups we have two modes of measurements: (1) Suns-$V_{OC}$ measurement, with switch

S1 open, and (2) Suns-$I_{SC}$ measurement, with switch S1 closed, thereby connecting the shunt resistance ($R_{SH}$) across the voltage read out.

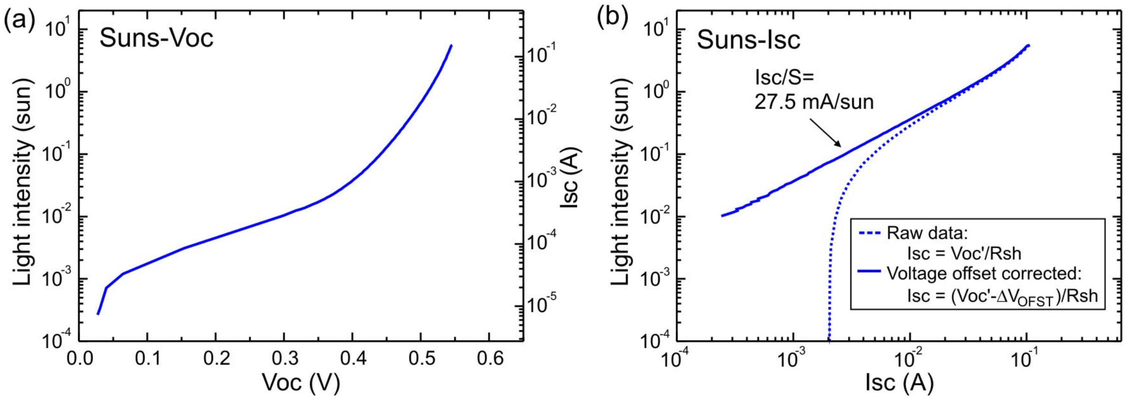


**Figure S2.** An example of (a) Suns-$V_{OC}$ curve. Short circuit current scale is shown on the right using the $I_{SC}$/S factor calculated from Suns-$I_{SC}$ measurement. (b) Suns-$I_{SC}$ measurement. Similar to Suns-$V_{OC}$ measurements except the measurement is shunted with $R_{sh}$ = 1Ω and with voltage offset correction of $\Delta V_{OFST} = 2.07\,\text{mV}$ .

The transient plot of the suns-$V_{OC}$ is shown in Figure S2. We could also plot this as $I_{SC}$ -$V_{OC}$ curves if we know the $I_{SC}$/sun factor that can be determined from suns-$I_{SC}$ measurement as shown in Figure S2(b).

We can perform the Sun-$I_{SC}$ measurement by shunting the $V_{OC}$ voltage read out by a small shunt resistance e.g. $R_{SH}$ = 1 Ω. The short circuit current at any intensity can be calculated as $I_{SC} = V_{OC}'/R_{SH}$ where $V_{OC}$' is the shunted "open circuit voltage" measured by the Sinton tool. The raw data of this Sun-$I_{SC}$ curve is shown as the dotted line in Figure S2(b). However there is a small voltage offset that usually occurs in the analog amplifier input stage of the data acquisition module. This offset voltage (~2 mV) is not negligible compared to the voltage being measured in the shunted condition ($V_{OC}$' ~ 0.1 – 100 mV). Thus the raw data of the Suns-$I_{SC}$ curve [dotted line, Figure S2(b)] does not look like a straight line as expected. We can extract this offset voltage in such a way that the corrected Suns-$I_{SC}$ curve shows a linear behavior, i.e. $I_{SC} = (V_{OC}' - \Delta V_{OFST})/R_{SH}$ . In the example shown in Figure S2(b), we obtain $\Delta V_{OFST} = 2.07\,\text{mV}$ . Given the "corrected Suns-$I_{SC}$" curve one can calculate the $I_{SC}$ /sun factor and calculate the $I_{SC}$ for any sun intensity as shown in the right scale of Figure S2(a), thus obtaining the $I_{SC}$-$V_{OC}$ plot. To minimize the voltage offset effect we could use higher $R_{SH}$; however this may distort the Suns-$I_{SC}$ curve at high light intensity [Figure S2(b)], as the voltage drop across the $R_{SH}$ becomes comparable with the $V_{OC}$.

The suns-$V_{OC}$ measurement has also been repeated for high performance CZTSSe devices with various bandgaps as shown in Figure S3 below. All the devices have carrier density < $10^{17}$ /cm$^3$,

as detected from drive level capacitance profiling technique [1]. In all curves we observe the suns-$V_{OC}$ bending behavior.

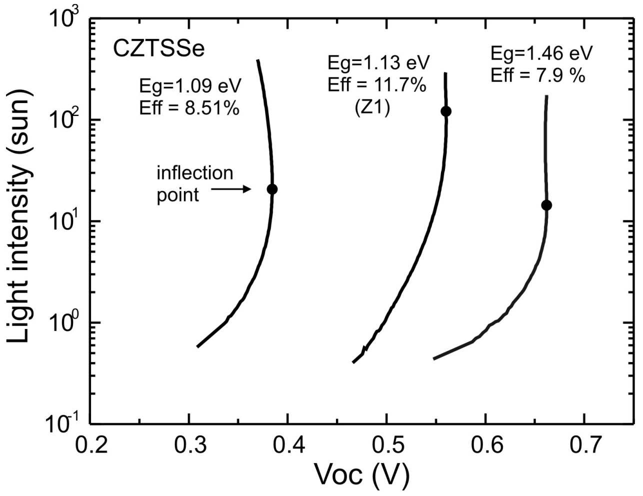


**Figure S3**. High intensity Suns-$V_{OC}$ curves of CZTSSe cells with increasing bandgap. The solid circles indicate inflection points where the ideality factor is zero. The open circles indicate the 1 sun intensity.

## *B. Low intensity suns-$V_{OC}$ (<1 sun) measurement using a Continuous Neutral Density Filter (CNDF)*

Besides using the Sinton tool we have also developed a technique to perform Suns-$V_{OC}$ measurement in a standard solar simulator as shown in Figure S4(a) thus allowing an immediate comparison of the $J_{SC}$-$V_{OC}$ curves and the standard light and dark $J$-$V$ curves. This system also allows low temperature measurements of the $J_{SC}$-$V_{OC}$ curves under the same solar simulator.

For the Suns-$V_{OC}$ sweep the solar simulator maintains a constant 1 sun output and its intensity is attenuated by using a special, custom-made large area continuous neutral density filter (CNDF) [2]. Large area CND filters are not commercially available; thus we fabricate them in-house using ink-jet printing on a common overhead projector transparency sheet. We first draw the radial gray scale pattern, print it and mount it on a black acrylic frame as shown in the inset of Figure S4(b). The filter is mounted on a stepper motor gearbox and can be rotated by a computer-controlled motor controller. The program is implemented in MATLAB.

For $J_{SC}$-$V_{OC}$ measurement, the system sets the baseline sun intensity to 1 sun and starts the CND filter at the open area position yielding the unattenuated, 1 sun illumination on the solar cell. The motor box then rotates the CND filer slowly towards the darker region and the system captures both $J_{SC}$ and $V_{OC}$ at every light intensity. We can achieve dynamic range of 1 to $10^{-4}$ sun using this setup and the $J_{SC}$-$V_{OC}$ data can be obtained with fine resolution for accurate ideality factor, $n_S$, extraction. The ideality factor is extracted from the asymptotic slope at the highest data point (at 1 sun) using Eq. 1.

The advantage of having an integrated $J_{SC}$-$V_{OC}$ setup into the existing solar simulator station is that we can measure the standard Light-$J$-$V$ and $J_{SC}$-$V_{OC}$ data in one sitting. This is not possible if the sun-$V_{OC}$ curve is captured in a separate system (e.g. the Sinton tool). Furthermore the measurement can also be conducted with a cryostat to obtain temperature dependent suns-$V_{OC}$ measurement as presented in Fig. 2.

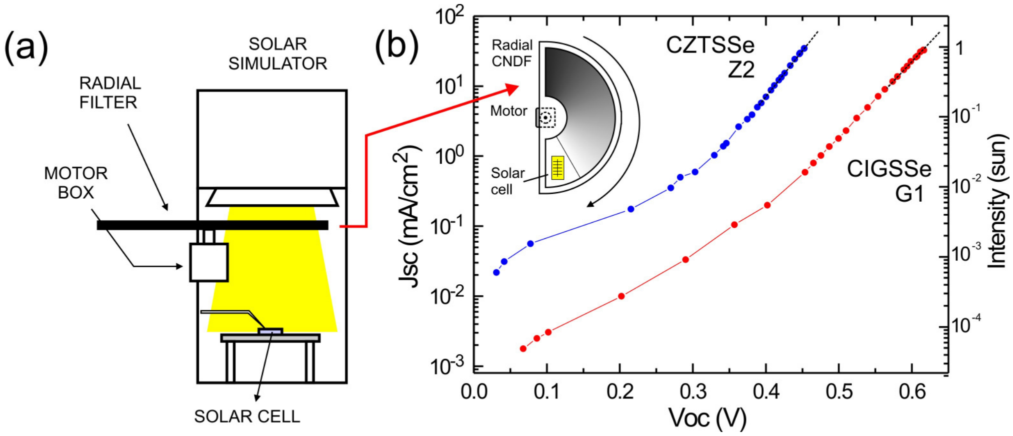


**Figure S4.** (a) Low intensity ($10^{-4}$ – 1 sun) Suns-$V_{OC}$ setup integrated into the standard solar simulator. (b) Sample Suns-$V_{OC}$ or $J_{SC}$-$V_{OC}$ data for CZTSSe cell "Z1" and a CIGSSe cell "G1". Inset: The radial CNDF that allows continuous light attenuation from 1 to ~$10^{-4}$ sun.

We can compare this "CNDF" technique and the Sinton's tool Suns-$V_{OC}$ measurement that we describe previously as shown in Figure S5. We observe that all measurements are consistent except they cover different ranges. This comparison also allows us to measure the absolute "sun" intensity at the solar cell in the Sinton tool by using the $J_{SC}$ at 1 sun measured from the solar simulator ($J_{SC}$-$V_{OC}$ data).

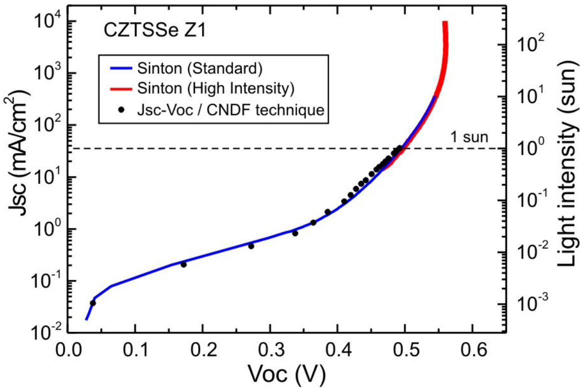


**Figure S5.** Comparison of Suns-$V_{OC}$ ($J_{SC}$-$V_{OC}$) measurements using the Sinton's tool and the CNDF technique.

## C. Ideality factor in a clean semiconductor solar cell

Here we derive the ideality factor of a solar cell made of clean semiconductor with no defect states in the band. The $V_{OC}$ is related to the quasi Fermi level separation at the front and the back contact:

$$V_{OC} = E_{Fn} - E_{Fp} \tag{S(1)}$$

The hole $E_{Fp}$ is mainly determined by the doping density:

$$E_{Fp} = E_i - k_B T / q \times \ln[(N_A + \Delta n) / n_i] \tag{S(2)}$$

where $n_i$ is the intrinsic carrier concentration and $E_i$ is the intrinsic Fermi level.

The electron $E_{Fn}$ will be mainly controlled by the light intensity. Here we have the generation rate proportional to the light intensity (or concentration factor S): $G = c_1 S$ , where $c_1$ is an arbitrary constant. Starting from Eq. 3, assuming a constant lifetime $\tau$ and clean density of states: $g(E) \propto \sqrt{E - E_C}$ we have:

$$G(S) = R = \int_0^{\infty} \frac{1}{1 + \exp[(E - E_{Fn}) / k_B T]} \frac{g(E)}{\tau(E,n)} dE , \tag{S(3)}$$

$$G(S) = c_1 S = n_i \exp[(E_{Fn} - E_i) / k_B T] / \tau = \Delta n / \tau \tag{S(4)}$$

$$E_{Fn} = E_i + k_B T / q \times \ln(\Delta n / n_i) \tag{S(5)}$$

where $\Delta n$ is the excess photogenerated electron density. Using Eq. S(1) we have: $V_{OC} = \frac{k_B T}{q} \ln\left(\frac{(N_A + \Delta n)\Delta n}{n_i^2}\right) \approx \frac{k_B T}{q} \ln\left(\frac{N_A \Delta n}{n_i^2}\right)$ since $N_A >> \Delta n$. From Eq. S(4) : $\Delta n = c_1 S \tau$ and using Eq. 1: $n_S = \left[V_T \, d\ln S / dV_{OC}\right]^{-1}$, we obtain $n_S = 1$.

## D. Circuit Model with Back Contact Diode

Our solar cell device can be modeled as a standard solar cell junction "PV" and a parasitic back contact junction "BC" shunted by a shunt resistance $R_{BC}$ as shown in Fig. 7(a). We can model the Suns-$V_{OC}$ behaviors of CZTSSe devices using the following relationship:

$$V_{OC}(S) = V_{OCA} - V_{OCB} = n_{1A} V_T \ln\left( \frac{S\, J_{L1A}}{J_{0A}} + 1 \right) - V_{OC,B} \qquad \text{S(6)}$$

$$S\, J_{L1B} = J_{0B}\left[\exp(V_{OCB} / n_{1B} V_T) - 1\right] + V_{OCB} / R_{BC} \quad , \qquad \text{S(7)}$$

where subscript A refers to the primary photovoltaic (PV) diode and B refers to the parasitic back contact diode. From the last equation we can solve for $V_{OCB}$ numerically as: $V_{OCB} = f(S, J_{L1B}, J_{0B}, n_{1B}, R_{BC})$.

We can fit this model into the experimental data as shown in Fig. 7. There are five independent parameters involved: $J_{L1A} / J_{0A}$, $n_{1A}$, $J_{L1B} / J_{0B}$, $n_{1B}$ and $R_{BC}$. First we extract $J_{L1A} / J_{0A}$ and $n_{1A}$ from the low sun intensity regime ($S$ < 1 sun) and then $J_{L1B} / J_{0B}$ and $n_{1B}$ from the high intensity regime by fitting $V_{OC} - V_{OCA}$ vs. $S$. In devices with poor back contact normally the $R_{BC}$ is not small (> 1 $\Omega$cm$^2$) and should be in order of the series resistance ($R_S$) of the device (if $R_{BC}$ is very small that means the back contact is good or ohmic). The Suns-Voc curve is not very sensitive to $R_{BC}$ when it is large (> 1 $\Omega$cm$^2$) [see Fig. 7(c)]. We could check the curve fitting result by substituting $R_{BC}$ ~ $R_S$ and observe almost no change in the calculated Suns-Voc curve. (For device Z2 using Sites' method for diode parameter extraction [3] we obtain $R_S$ = 5.2 $\Omega$cm$^2$).

For the data as shown in Fig. 6(a) and performing a numerical curve-fitting, we obtain: $n_{1A} = 0.82$, $J_{L1A} / J_{0A} = 4.0 \times 10^9$, $n_{1B} = 1.7$ and $J_{L1B} / J_{0B} = 0.71$ and $R_{BC}$ ~5 $\Omega$cm$^2$. These parameters provide a good fit to the experimental data as shown in Fig. 7(a). We observe that the dark reverse saturation current of the back contact ($J_{0B}$) is much larger (relative to its photocurrent $J_{L1}$) than that of the primary diode ($J_{0A}$), indicating that this junction is very leaky– which is expected for a junction that is originally intended to be an ohmic contact.

## *REFERENCES*


[1] J. T. Heath, J. D. Cohen, and W. N. Shafarman, *Bulk and metastable defects in $CuIn_{1-x}Ga_xSe_2$ thin films using drive-level capacitance profiling*, J. Appl. Phys. **95**, 1000 (2004).

[2] O. Gunawan and B. Lei, Solar cell characterization system with an automated continuous neutral density filter, US 20120223733 A1 (2012).

[3] J. R. Sites and P. H. Mauk, *Diode quality factor determination for thin-film solar cells*, Sol. Cells **27**, 411 (1989).
